# Supplementary material for: Evaluating Large Language Model with Knowledge Oriented Language Specific Simple Question Answering
Source: arXiv:2505.16591 source file (2025-05-22)
Supplement: Supplementary file 1 [file appendix_example_table.tex]

\begin{table*}[]
\centering
\resizebox{\textwidth}{!}{
\begin{tabular}{c|c|c|c|c|c}
\hline
\textbf{Wiki-url}   & \textbf{Soure Texts}  & \textbf{domain} & \textbf{triple} & \textbf{Question-Answer Pairs} & \textcolor{blue}{\textbf{translation to EN}} \\
\hline

https://zh.wikipedia.org/wiki/何家慧 &
\begin{tabular}[c]{@{}p{5cm}@{}} 何家慧1978年加入乐坛推出个人大碟《小白船》，1988年曾以部头形式签约亚洲电视演出电视剧，后退出娱乐圈，并移民至加拿大温哥华\end{tabular} & 
\begin{tabular}[c]{@{}p{1.8cm}@{}}zh-specific\end{tabular} &
\begin{tabular}[c]{@{}p{5cm}@{}}["何家慧", "移民至", "温哥华"]\end{tabular} & 
\begin{tabular}[c]{@{}p{3.5cm}@{}}Question: 何家慧移民至哪个城市？\\ Answer: 温哥华\end{tabular} & 
\begin{tabular}[c]{@{}p{3.5cm}@{}}\textcolor{blue}{Question:To which city did He Jiahui immigrate?}\\ \textcolor{blue}{Answer: Vancouver}\end{tabular} \\
\hline

https://zh.wikipedia.org/wiki/光明节 &
\begin{tabular}[c]{@{}p{5cm}@{}} 光明节,又称修殿节、献殿节、烛光节、哈努卡节、马加比节等，是一个犹太教的节日\end{tabular} & 
\begin{tabular}[c]{@{}p{1.8cm}@{}}zh-general\end{tabular} &
\begin{tabular}[c]{@{}p{5cm}@{}}["光明节", "是节日", "犹太教"]\end{tabular} & 
\begin{tabular}[c]{@{}p{3.5cm}@{}}Question: 光明节是哪个宗教的节日？\\ Answer: 犹太教\end{tabular} & 
\begin{tabular}[c]{@{}p{3.5cm}@{}}\textcolor{blue}{Question:Which religion celebrates Hanukkah?}\\ \textcolor{blue}{Answer: Judaism}\end{tabular} \\
\hline

https://zh.wikipedia.org/wiki/光明节 &
\begin{tabular}[c]{@{}p{5cm}@{}} 光明节,又称修殿节、献殿节、烛光节、哈努卡节、马加比节等，是一个犹太教的节日\end{tabular} & 
\begin{tabular}[c]{@{}p{1.8cm}@{}}zh-general\end{tabular} &
\begin{tabular}[c]{@{}p{5cm}@{}}["光明节", "是节日", "犹太教"]\end{tabular} & 
\begin{tabular}[c]{@{}p{3.5cm}@{}}Question: 光明节是哪个宗教的节日？\\ Answer: 犹太教\end{tabular} & 
\begin{tabular}[c]{@{}p{3.5cm}@{}}\textcolor{blue}{Question:Which religion celebrates Hanukkah?}\\ \textcolor{blue}{Answer: Judaism}\end{tabular} \\
\hline

\end{tabular}}
\caption{Examples of KolasSimpleQA}
\label{tab:husimleqa_examples}
\end{table*}
